# Supplementary material for: Mapping the Privacy-Utility Tradeoff in Mobile Phone Data for Development
Source: arXiv:1808.00160 source file (2018-08-01)
Supplement: Supplementary file 1 [file Additional_file_1_--_Supp_figures_on_reidentification.pdf]

---

# Mapping the Privacy-Usefulness Tradeoff in Mobile Phone Metadata for Development

A. Noriega-Campero, Yves A. de Montjoye, Alex Rutherford, Oren Lederman, and Alex Pentland

## Additional file 1: Supplementary figures on reidentification

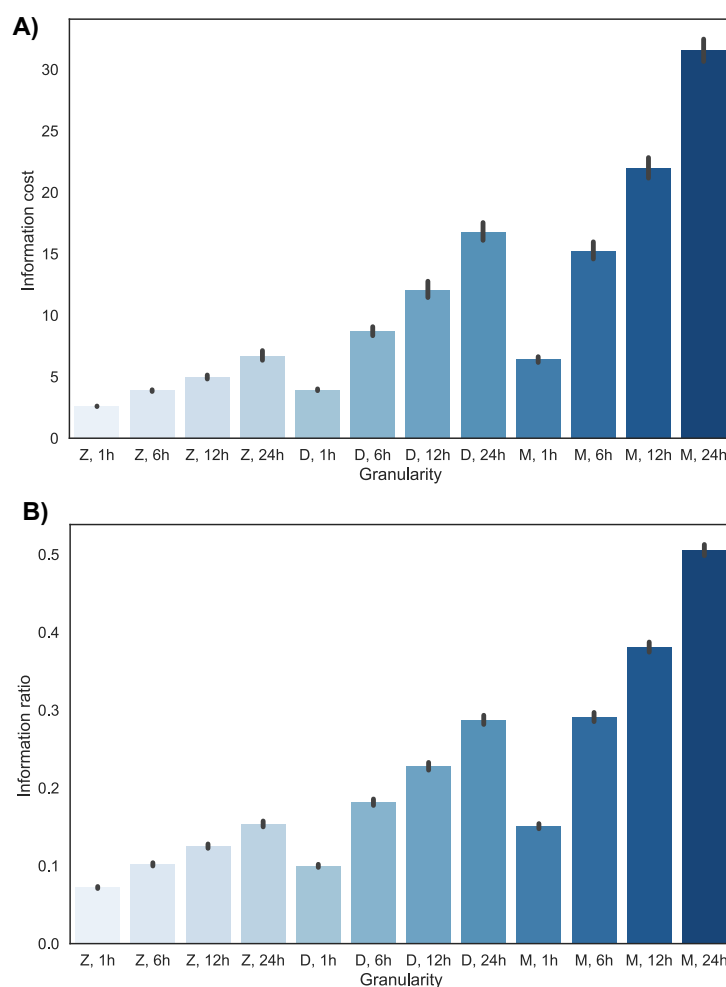

**Fig 1.** Reidentification results for datasets at varying levels of spatial and temporal granularity: *information cost*, and *information ratio*. Grey bars indicate bootstrapped 95% confidence intervals.

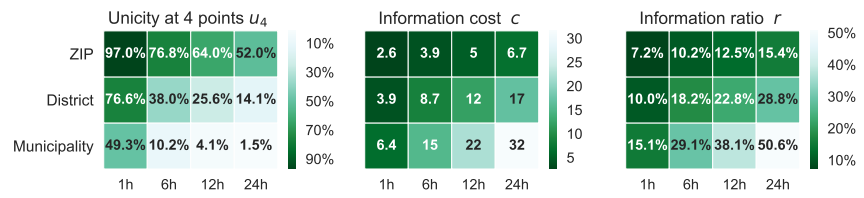

**Fig 2.** Reidentification results for datasets at varying levels of spatial and temporal granularity. Comparison of *unicity*, *information cost*, and *information ratio*.
